# Supplementary material for: Completely Reachable Automata, Primitive Groups and the State Complexity of the Set of Synchronizing Words
Source: arXiv:2007.09104 source file (2020-11-28)
Supplement: Supplementary file 1 [file appendix.tex]

Here we collect some proofs not given in the main text. % here, we collect? komma

\subsection{Proof of Lemma~\ref{lem:compl_reach_implies_max_Syn_2sets} (See page~\pageref{lem:compl_reach_implies_max_Syn_2sets})}
\complreachimpliesmaxSyntwosets*

\subsection{Proof of Corollary~\ref{cor:poly_alg_max_sync} (See page~\pageref{cor:poly_alg_max_sync})}
\polyalgmaxsync*

\subsection{Proof of Proposition~\ref{prop:groups_max_sc_implies_compl_reach} (See page~\pageref{prop:groups_max_sc_implies_compl_reach})}
\groupsmaxscimpliescomplreach*

\subsection{Proof of Corollary~\ref{cor:max_sc_implies_primitive} (See page~\pageref{cor:max_sc_implies_primitive})}
\maxscimpliesprimitive*

\subsection{Proof of Proposition~\ref{prop:2_hom_perm_group} (See page~\pageref{prop:2_hom_perm_group})}
\twohompermgroup*

\subsection{Proof of Proposition~\ref{prop:k_reachable_implies_k_hom} (See page~\pageref{prop:k_reachable_implies_k_hom})}
\kreachableimplieskhom*
